# Supplementary material for: Invariant Information Clustering for Unsupervised Image Classification and Segmentation
Source: arXiv:1807.06653 source file (2019-08-22)
Supplement: Supplementary file 1 [file appendix.tex]

\subsection{Relation to other clustering methods}\label{s:discuss}

\paragraph{Information bottleneck.}

IID is related to \emph{multivariate information bottleneck} (MIB)~\cite{friedman2001multivariate,wang10information}. MIB can be described as optimizing a variant of~\cref{e:info_orig} given by:
\begin{multline*}
\min_{\Phi} 
I(\bx,\Phi(\bx)) + I(\bx',\Phi(\bx')),
\\
\text{s.t.\ }
I(\bx,\bx') = I(\Phi(\bx),\Phi(\bx')).
\end{multline*}
In MIB, $\Phi$ is a deterministic function of the data, so that $I(\bx,\Phi(\bx))=H(\Phi(\bx))$ is simply the entropy of the representation. Hence, MIB seeks for the lowest entropy representation that preserves the mutual information between $\bx$ and $\bx'$, whereas IID bounds the representation entropy via the $\ln C$ bottleneck and maximises mutual information.

\paragraph{Generative clustering.}

Generative clustering methods such as K-means depend on the metric which is defined in the data space, whereas information-based clustering methods such as IID are invariant to the choice of metric.
Formally, and barring pathological cases, if $f : \mathcal{X}\rightarrow\mathcal{X}$ is a bijective mapping of the data space onto itself, then information $I(f(\bx),f(\bx')) = I(\bx,\bx')$ is preserved, whereas distances $d(f(\bx),f(\bx')) \not= d(\bx,\bx')$ are not.

This is a profound difference between these two approaches to clustering.
Being invariant to the metric is partially an advantage, as clustering works the same regardless of the particular representation of the input data, but it can also be a disadvantage, as sometimes the metric defined in data space carries useful prior knowledge about the problem.
